# Supplementary material for: Granger Causality Networks for Categorical Time Series
Source: arXiv:1706.02781 source file (2017-06-08)
Supplement: Supplementary file 1 [file appendix2.tex]

\section{Appendix 2: High Dimensional Estimation for mLTD}
%\subsection{upper bounding covering proof}
%Let $N = N \text{pr} (\gamma \delta_m; \mathbb{B}_m^{'};||.||_T)$ be the minimal $\gamma \delta_m$ covering of $\mathcal{B}_m^{'}$ in norm $||.||_T$. We want to upper bound this covering number such that it holds for all $x$. This number is random as both the norm $||.||_T$, and the set $\mathcal{B}_m^{'}$ depend on $x$. For each $x$ $N$ is upper bounded by:
%\begin{align}
%N \leq \exp(\frac{2048}{\gamma^2 \delta_m^2} U^2 \rho_m \log(2M)).
%\end{align}
%Let $N^* = \lceil \exp(\frac{2048}{\gamma^2 \delta_m^2} U^2 \rho_m \log(2M)) \rceil$. Then let  $N^* \text{pr} (\gamma \delta_m; \mathbb{B}_m^{'};||.||_T)$ be a covering with $N^{*}$ elements, which is always possible since it is always bigger than the minimal covering. We have that for any $\Delta_m^k$ in the covering:
%\begin{align}
%P\left(\delta_m^2 - ||\Delta_m^k||^2_T > (1 - \frac{\xi}{2} \omega) \delta_m^2\right) \leq \exp(- \frac{c \omega^2}{\rho_m^2} T)
%\end{align}
%So that a union bound gives:
%\begin{align}
%P\left(\max_{k = 1,2, \ldots, N^*} \delta_m^2 - ||\Delta_m^k||_T^2 > (1 - \frac{\xi}{2} \omega) \delta_m^2\right) \leq \exp \left(\log \left(\lceil \exp(\frac{2048}{\gamma^2 \delta_m^2} U^2 \rho_m \log(2M)) \rceil \right) - \frac{c \omega^2}{\rho_m^2} T \right)
%\end{align}
\subsection{Introduction}
This section of the Appendix develops estimation rates for inference in a autoregressive categorical GLM. The results are based on generalizations of results for autoregressive GLMs given in \cite{}. The original set of bounds in \cite{} for high dimensional estimation in multivariate GLMs was only for time series with one dimensional natural parameters, like Poisson or Bernoilli autoregressive time series. In the categorical setting there are $k - 1$ natural parameters for each time series; thus we first extend the results of \cite{} to autoregressive GLMs with multivariate natural parameters and vector outputs and then apply these results to establish high dimensional estimation rates for the multivariate categorical autoregressive GLM (mLTD).
\subsection{Autoregressive GLMs with vector valued outputs and natural parameters}
To derive the results, we first derive general results for auto-regressive GLMs. Consider the generalized linear autoregressive model with multiple outputs:
\begin{align}
X_{t+1,m} | X_t \sim p(\nu_m + A_m^* X_t)
\end{align}
where $X_{t+1,m} \in \mathbb{R}^k$ is the $m$th observation of $X_{t+1} \in \mathbb{R}^{k*M}$ and $A_m \in [a_{min},a_{max}]^{k x kM}$ is an unknown parameter vector where
\begin{align}
A_m = (A_{1,m}, \ldots, A_{M,m})
\end{align}
with $A_{1,m} \in R^{k \times k}$, $\nu_m \in [\nu_{min},\nu_{max}]^k$ is a known, constant offset parameter, and $p$ is an exponential family probability distribution. Specifically, $X \sim p(\theta)$ means that the distribution of the vector $X$ is associated with the density $p(x|\theta) = h(x) \text{exp}(\phi(x)^T \theta - Z(\theta))$ where $\theta$ is a vector variate parameter and $Z$ is the log partition function, $\phi(x)$ is the sufficient statistic of the data, and $h(x)$ is the base measure of the distribution. Examples that fit this are the multivariate normal distribution and multinomial distributions. The conditional covariance is dependent on the previous data instead of being constant equal to the noise covariance.

The conditional distribution is given explicitly as:
\begin{align}
p(X_{t+1}|X_t) = \prod_{m=1}^{M} h(X_{t+1,m}) \text{exp}(\phi(X_{t+1,m})^T (\nu_m + A^*_m X_t) - Z(\nu_m + A^*_m X_t))
\end{align}
We observe $T$ samples $(X_t)_{t=0}^{T}$ and our goal is to infer $A^*$. In high dimensional setting we have structural assumptions on $A^*$. Let 
\begin{align}
S := \{(l,m) \in {1, \ldots, M}^2: A^*_{l,m} \neq 0\}.
\end{align}
where $A^*_{l,m}$ is the $l$th submatrix of $A_m$. We assume the matrix $A^*$ is s-sparse meaning that $|S| \leq s$. Furthermore, let $\rho_m$ be the number of nonzero sub-matrices $A^*_{l,m}$ in $A_m$ and $\rho := \max_m \rho_m$.

We estimate $A^*$ via a constrained maximum likelihood solving:
\begin{align}
\min_A \frac{1}{T} \sum_{t = 0}^{T-1} \left(Z(\nu_m + A_m X_t) - A_m X_t \phi(X_{t+1},m)\right) + \lambda ||A_m||_1
\end{align}
or with a group lasso penalty
\begin{align}
\min_A \frac{1}{T} \sum_{t = 0}^{T-1} \sum_{m=1}^{M} \left(Z(\nu_m + A_m X_t) - A_m X_t \phi(X_{t+1},m)\right) + \lambda \sum_{l = 1}^{M} ||A_{l,m}||_F
\end{align}
For notational simplicity, we define $||A||_{\G} = \sum_{l = 1}^{M} ||A_{l,m}||_F$.

\subsection{Main Result}
\paragraph{Assumption 1.} We assume that for any realization of the process there exists a subset of the observations $\{X_{\mathcal{T}_t}\}_{t=1}^{\mathcal{T}}$ for $\mathcal{R} \subset \{0, 1, \ldots, T-1\}$ that satisfies:
\begin{enumerate}
\item There exists a constant $U$ such that $U \geq \text{max} ||X_t||_{\infty}$ where $U$ is independent of $T$.
\item $Z()$ is $\sigma$-strongly convex on a domain determined by $U$:
\begin{align}
Z(x) \geq Z(y) + Z'(y)(x-y) + \frac{\sigma}{2}||x - y||_2^2
\end{align}
for all $x,y \in [-\tilde{\nu} - 9 \rho \tilde{a} {\bf 1} U, \tilde{\nu} + 9 \rho \tilde{a} {\bf 1} U ] $ where $\tilde{nu} = \max(|\nu_{min}|,|\nu_{max}|)$ and $\tilde{a} = \max{|a_{min}|,|a_{max}|}$, where $\sigma$ is independent of $T$. 
\item The smallest eigenvalue of $\Gamma_t = E[X_{\mathcal{T}} X_{\mathcal{T}}^T|X_{\mathcal{T}_{t-1}}]$ is lower bounded by $\omega > 0$, which is independent of $T$. 
\end{enumerate}

Define the constant $\beta \leq \frac{|\mathcal{T}|}{T}$, which will be determined by the constant $U$, and can be set such that $\beta$ is very close to 1.

\subsubsection{Convergence Rates}
 
\begin{ntheorem} \label{glm_thm}
Assume $\frac{\lambda}{2} \geq \max_{1 \leq m \leq M} \left|\left| \frac{1}{T} \sum_{t=0}^{T-1} \epsilon_{t,m} X_t^T \right|\right|_{\G,\infty}$, and let $\hat{A}$ be the RMLE for a process which obeys Assumption 1. Then for any $A_m$ and for any $\delta \in (0,1)$, which probability $(1 - \delta)$
\begin{align}
||\hat{A}_m - A^*_m||_{2}^{2} \leq \frac{144}{\beta^2 \sigma^2 \omega^2} \rho_m k^2 \lambda^2 
\end{align}
for $T \geq \frac{c \rho_m^2 k^4}{\omega} \left(\frac{\rho_m k^2 \log(2M)}{\omega^2} + \log(\frac{1}{\delta}) \right)$  where $c$ is independent of $M, T, \rho$ and $s$.  
\end{ntheorem}
\subsubsection{Proof of Theorem \ref{glm_thm}}
The optima satisfies:

\begin{align}
\frac{1}{T} \sum_{t = 0}^{T-1} Z(\nu_m + \Ahm X_t) - (\Ahm X_t)^T \phi(X_{t+1,m}) + \lambda ||\Ahm||_{G} \\
\leq \frac{1}{T} \sum_{t=0}^{T-1} Z(\nu_m + \Asm X_t) + (\Asm X_t)^T \phi(X_{t+1,m}) + \lambda ||\Asm||_G
\end{align}
define $\epsilon_{t,m} = \phi(X_{t+1,m}) - E(\phi(X_{t+1,m})|X_t))$, which is a conditionally zero mean random variable. We know that $E(\phi(X_{t+1,m})|X_t)) = Z'(\nu_m + \Asm X_t)$, and so that $\phi(X_{t+1,m} = Z'(\nu_m + \Asm X_t) + \epsilon_{t,m}$, giving:
\begin{align}
\frac{1}{T} \sum_{t = 0}^{T - 1} Z(\nu_m + \Ahm X_t) - (\Ahm X_t)^T (Z'(\nu_m + \Asm X_t) + \epsilon_{t,m}) + \lambda ||\Ahm||_G \\
\leq \frac{1}{T} \sum_{t = 0}^{T - 1} Z(\nu_m + \Asm X_t) - (\Asm X_t)^T (Z'(\nu_m + \Asm X_t) + \epsilon_{t,m}) + \lambda ||\Asm||_G
\end{align}
Moving terms gives:
\begin{align}
\frac{1}{T} \sum_{t = 0}^{T-1} B_{Z}(\nu_m + \Ahm Xt || \nu_m + \Asm X_t) \\
\leq \left|\frac{1}{T} \sum_{t=0}^{T-1} \epsilon_{t,m}^T \Delta_m X_t\right| + \lambda \left(||\Asm||_G - ||\Ahm||_G \right)
\end{align}
where $\Delta = \Ahm - \Asm$. We upper bound the right hand side of the inequality as:
\begin{align}
\frac{1}{T} \sum_{t=0}^{T-1} B_{Z} (\nu_m + \Ahm X_t || \nu_m + \Asm X_t) &\leq \left|\frac{1}{T} \sum_{t = 0} \epsilon_{t,m}^T \Delta_m X_t \right| + \left(||\Asm||_{\G} - ||\Ahm||_{\G} \right) \\
&= \left|\frac{1}{T} \sum_{t = 0} \epsilon_{t,m}^T \Delta_m X_t \right| + \lambda(||\Asms||_{\G} - ||\Ahms||_{\G} - ||\Ahmsc||_{\G}) \\
&\leq \left|\frac{1}{T} \sum_{t = 0} \epsilon_{t,m}^T \Delta_m X_t \right| + \lambda ||\Delta_{m,S}||_{\G} - \lambda||\Delta_{m,S^c}||_{\G} \\
&\leq \textcolor{red}{||\Delta||_{\G} \left|\left| \frac{1}{T} \sum_{t=0}^{T-1} \epsilon_{t,m} X_t^T\right|\right|_{\G,\infty} + \lambda ||\Delta_{m,S}||_{\G} - \lambda||\Delta_{m,S^c}||_{\G}}
\end{align}
where $||Y||_{\G,\infty}$ is the maximum of the Froebenius norm of the groups in $Y$, given by 
\begin{align}
||Y||_{\G,\infty} = \max_{i = 1, \ldots, M} ||Y_{j}||_F
\end{align}
where $Y_{j}$ is the $j$th block matrix of $Y$. $S$ is the true support of $\Ahm$ and we have used the decomposability of $|| . ||_{\G}$. The decomposability means that we have the property
\begin{align}
||X||_{\G} = ||X_S||_{\G} + ||X_{S^c}||_{\G}.
\end{align}
Note that $\left|\left| \frac{1}{T} \sum_{t=0}^{T-1} \epsilon_{t,m} X_t^T \right|\right|_{\G,\infty} \leq \max_{1 \leq m \leq M} \left|\left| \frac{1}{T} \sum_{t=0}^{T-1} \epsilon_{t,m} X_t^T \right|\right|_{\G,\infty}$. Under the assumption that $\frac{\lambda}{2} \geq \max_{1 \leq m \leq M} \left|\left| \frac{1}{T} \sum_{t=0}^{T-1} \epsilon_{t,m} X_t^T \right|\right|_{\G,\infty}$ and by the non-negativity of the Bregman divergence on the left hand side of the inequality, we have that
\begin{align}
0 \leq \frac{\lambda}{2} ||\Delta_m||_{\G} + \lambda ||\Delta_{m,S}||_{\G} - \lambda || \Delta_{m,S^c}||_{\G}.
\end{align}
Using the decomposability of the norm, this inequality implies that we have $||\delta_{m,S^c}||_{G} \leq 3 || \delta_{m,S}||_{\G}$. Since $||\Delta_{m,S^c}||_{\G} \leq 3 ||\Delta_{m,S}||_{\G}$, $||\delta_m||_{\G} \leq 4 || \Delta_{m,S}||_{\G}$ and consequently 

\begin{align}
\textcolor{red}{||\Delta_m||_{\G} \leq 4 \sum_{j \in S} ||\Delta_{m,j}||_{F} \leq 8 \rho_m k \tilde{a}}
\end{align}

%Using this inequality and the fact that ||\A
By Assumption 1, $Z$ is $\sigma$-strongly convex, and therefore on $\mathcal{T}$ it is true that $B_{Z}(\nu_m \Ahm X_t || \nu_m + \Asm X_t) \geq \frac{\sigma}{2} ||\Delta_m X_t||_2^2$ and $B_{Z}(\nu_m \Ahm X_t || \nu_m + \Asm X_t) \geq 0$ on the rest of the time indices. Therefore,
\begin{align}
\frac{\sigma}{2 T} \sum_{t \in \mathcal{T}} ||\Delta_m X_t||^2_2 \leq \frac{\lambda}{2} || \Delta_m||_{\G} + \lambda || \Delta_{m,S}||_{\G} - \lambda || \Delta_{m,S^c}||_{\G}.
\end{align}
Define $||\Delta_m||^2_{T} = \frac{1}{T} \sum_{t \in \mathcal{T}} ||\Delta_m X_t||^2_2$. We have that
\begin{align}
\frac{\sigma}{2}||\Delta_m||_T^2 \leq \frac{\lambda}{2} ||\Delta_m||_{\G} + \lambda ||\Delta_{m,S}||_{\G} - \lambda || \Delta_{m,S^c}||_{\G} \leq \frac{3 \lambda}{2} ||\Delta_{m,S}||_{\G}.
\end{align}
Define the cone on which the matrix $\Delta_m$ must be defined:
\begin{align}
\mathcal{B}_{m,S} = \{\Delta_m | ||\Delta_{m,S^c}||_{\G} \leq 3 || \Delta_{m,S}||_{\G}\},
\end{align}
and restrict ourselves to studying properties of matrices in that set. By Cauchy-Shwartz we have that $||\Delta_{m,S}||_{\G} \leq \sqrt{\rho_m} ||\Delta_m||_F$ where $\rho_m$ is the number of non-zeros of $\Asm$. We then have that 
\begin{align}
||\Delta_m||_{T}^2 \leq \frac{3}{\sigma} \lambda \sqrt{\rho_m} ||\Delta_m||_F = \delta_m|| \Delta_m||_F.
\end{align}
where $\delta_m = \frac{3}{\sigma} \sqrt{\rho_m}$. 

Now consider three cases: if $||\Delta_m||_T \geq ||\Delta||_2$, then $\max(||\Delta_m||_T, ||\Delta_m||_2) \delta_m$. On the other hand if $||\Delta_m||_T \leq ||\Delta_m||_2$ and $||\Delta_m||_2 \leq \delta_m$ then $\max(||\Delta_m||_T, ||\Delta_m||_2) \leq \delta_m$.  

The final case to consider is |$|\Delta_m||_T \leq ||\Delta_m||_2$ and $||\Delta_m \geq \delta_m$. Define the following set:
\begin{align}
\mathcal{B}_m(\delta_m) = \{ \Delta_m \in \mathcal{B}_{m,S} | \,\, ||\Delta_m||_T \leq ||\Delta_m||_2, ||\Delta_m||_2 \geq \delta_m \}
\end{align}
and 
\begin{align}
\mathcal{B}_m(\delta_m) = \{ \Delta_m \in \mathcal{B}_{m,S} | \,\, ||\Delta_m||_T \leq ||\Delta_m||_2, ||\Delta_m||_2 = \delta_m \}
\end{align}

We will show that for $|\delta \in \mathcal{B}_m(\delta_m)$, we have $||\Delta_m||_T^2 \geq \kappa ||\Delta_m||_F^2$ for some $\kappa \in (0,1)$ with high probability. We claim its enough to show that $||\Delta_m||^2_T \geq \kappa ||\Delta_m||_2^2$ is true on $\mathcal{B}^{'}_m(\delta_m)$ with high probability. In particular, given an arbitrary non-zero $\Delta_m \in \mathcal{B}_m(\delta_m)$, consider the rescaled vector $\tilde{\Delta_m} = \frac{\delta_m}{||\Delta_m||_2} \Delta_m$. Since $\Delta \in \mathcal{B}_m(\delta_m)$, we have $\tilde{\delta_m} \in \mathcal{B}_m(\delta_m)$ and $||\tilde{\Delta}||_2 = \delta_m$ by construction. Therefore, if $|| \tilde{\Delta}_m||_{T}^2 \geq \kappa ||\tilde{\Delta}_m||^2_2$ is true, then $||\Delta||_T^2 \geq \kappa ||\Delta_m||^2_2$ is also true. Alternatively, if we define the random vaiable $\mathcal{Z}_T(\mathcal{B}_m^{'}) = \sup_{\Delta_m \in \mathcal{B}_m^{'}(\delta_m)}\{\delta_m^2 - ||\Delta_m||_T^2\}$. 

Recall that the emprical norm is $||\Delta_m||_2^T = \frac{1}{T} \sum_{t \in \mathcal{T}} ||\Delta_m X_t||_2^2$. Let $\mathcal{N} = N \text{pr}(\gamma \delta_m ; \mathcal{B}_m^{'}; ||.||_T)$ denote the proper covering number of $\mathcal{B}_m^{'}$ in $||.||_T$ norm. Now let $\Delta_m^1, \Delta_m^2, \ldots, \Delta_m^{\mathcal{N}}$ be a minimal $\gamma \delta_m$ proper covering of $\mathcal{B}_m^{'}$ so that for all $\Delta_m \in \mathcal{B}_m^{'}$, there is a $\Delta_m^k$ in the covering set such that $||\Delta_m^k - \Delta_m||_T \leq \gamma \delta_m$. We can write
\begin{align}
\delta^2_m - ||\Delta_m||_T^2 = (\delta^2_m - ||\Delta_m^k||_T^2) + (||\Delta_m^k||_T^2 - ||\Delta_m||_T^2)
\end{align}
for any $k \in \{1,2,\ldots, \mathcal{N}\}$. By the Cauchy-Schwarz inequality, we have
\begin{align}
\frac{1}{T} \sum_{t \in \mathcal{T}} ||\Delta_m^k X_t||_2^2 - ||\Delta_m X_t||_2^2 = \frac{1}{T} \sum_{t \in \mathcal{T}} X^T_t (\Delta_m^k - \Delta_m)^T(\Delta_m^k + \Delta_m) X_t \\
\leq ||\Delta_m^k - \Delta_m||_T ||\Delta_m^k + \Delta_m||_T
\end{align}
By the choice of covering, we have $||\Delta_m^k - \Delta_m||_T \leq \gamma \delta_m$. On the other hand, by the definition of $\mathcal{B}'_m$ we have $||\Delta_m||_T \leq \delta_m$ and $||\Delta_m^k||_T \leq \delta_m$ so 
\begin{align}
\Delta_m^k + \Delta_m||_T \leq 2 \delta_m.
\end{align}
Overall, we have establisshed that $\frac{1}{T} \sum_{t \in \mathcal{T}} ||\delta_m^k X_t||_2^2 - \frac{1}{T} \sum_{t \in \mathcal{T}} ||\Delta_m X_t||_2^2 \leq 2 \gamma \delta_m^2$. Hence we have:
\begin{align}
\mathcal{Z}_T(\mathcal{B}_m) \leq \max_{1 \leq k \leq \mathcal{N}} \{\delta_m^2 - ||\Delta_m^k||_T^2\} + 2 \gamma \delta^2_m,
\end{align}
where $\mathcal{N} = N \text{pr} (\gamma \delta_m ; \mathcal{B}_m^{'} ||.||^2_{T})$. For any $\Delta_m^k$ in our covering set, we use the definition of $\psi$ and Lemma 5,
\textcolor{red}{
\begin{align}
\mathbb{P}(\delta_m^2 - ||\Delta_m^k||_T^2 > (1 - \frac{\psi}{2}\omega) \delta_m) > (1 - \frac{\psi}{2}\omega) \delta_m^2) \leq \mathbb{P}(\delta_m^2 - ||\Delta_m^k||_T^2 > (1 - \frac{|\mathcal{T}|}{2 T} \omega) \delta_m^2) \leq \exp\left(- \frac{c \omega^2}{\rho^2_m k^4} T\right)
\end{align}}
where $\omega$ is the minimum eigen value of $E[X_{\tilde{T}_t} X_{\tilde{T}_t}^T | X_{\tilde{T}_{t-1}}]$ for any $\mathcal{T}_t$ and $\mathcal{T}_{t-1}$ which are consecutive elements of $\mathcal{T}$ and which holds by assumption. 

A union bound gives,
\begin{align}
P\left(\max_{k = 1,\ldots, \mathcal{N}} \delta_m^2 - ||\Delta_m^k||^2_T > (1 - \frac{\psi}{2} \omega) \delta_m^2 \right) \leq \exp \left(\log N_{pr}(\gamma \delta_m ; \mathcal{B}_m^{'}, ||.||_T ) - c \frac{\omega^2}{\rho_m^2 k^4} T \right).
\end{align}
We now bound the covering number $\log N_{pr}(\gamma \delta_m ; \mathcal{B}_m^{'}, ||.||_T )$. This is upper bounded by $\log N_{pr}(\frac{\gamma \delta_m}{2} ; \mathcal{B}_m^{'}, ||.||_T )$, which we upper bound. Define the zero mean Gaussian process $\{W_{\Delta}\}_{\Delta \in \mathcal{B}_m^{'}}$ by $W_{\Delta_m} = \frac{1}{\sqrt{T}} \sum_{t \in \mathcal{T}} w_t^T \Delta_m X_t$ where $\{w_t\}$ are i.i.d $k$ variate Gaussian random variables with zero mean and identity covariance.

 We have $\text{Var}[W_{\Delta_m} - W_{\Delta'_m})] = ||\Delta_m - \Delta_m^{'}||_T^2$. By the Sudakov minoration, for all $\gamma, \delta_m > 0$ we have $(\gamma \delta_m / 2) \sqrt{\log N(\gamma \delta_m/2, \mathcal{B}_m', ||>||_T)} \leq 4 E_w[\text{sup}_{\Delta_m \in \mathcal{B}_m^{'}} \frac{1}{\sqrt{T}} \sum_{t \in \mathcal{T}} w_t^T \Delta_m X_t]$, giving in the upper bound:
 \begin{align}
 \sqrt{\log N(\gamma \delta_m/2, \mathcal{B}_m', ||>||_T)} \leq \frac{8}{\gamma \delta_m} E_w[\text{sup}_{\Delta_m \in \mathcal{B}_m^{'}} \frac{1}{\sqrt{T}} \sum_{t \in \mathcal{T}} w_t^T \Delta_m X_t]
 \end{align}
 We can bound the Gaussian complexity as:
 \begin{align}
 \frac{1}{\sqrt{T}} \sum_{t \in \mathcal{T}} w_t^T \Delta_m X_t \leq \left|\left|\frac{1}{\sqrt{T}} \sum_{t \in \mathcal{T}}  w_t X_t^T \right| \right|_{G,\infty}||\Delta_m||_{G}
 \end{align}
 Since $\Delta \in \mathcal{B}_{m}^{'}(\delta_m)$, we have thate $||\Delta_m||_{\G} = || \Delta_{m,\mathcal{S}}||_{\G} + || \Delta_{m,\mathcal{S}^c}||_{\G} \leq 4 || \Delta_{m,\mathcal{S}}||_{\G}$ and $|| \Delta_{m,\mathcal{S}}||_{\G} \leq \sqrt{\rho_m} ||\Delta_{m,\mathcal{S}}||_F \leq || \Delta_{m}||_{\G} = \sqrt{\rho_m} \delta_m$. This combined with Lemma \label{gauss_comp} gives:
 \begin{align}
 \log N(\gamma \delta_m.2, \mathcal{B}', ||.||_T) &\leq \frac{2048}{\gamma^2 \delta_m^2} U^2 k^2 \log (2 M k^2) ||\Delta_{m,\mathcal{S}}||_{\G} \\
 &\leq \frac{2048}{\gamma^2} U^2 k^2 \rho_m \log(2 M k^2).
 \end{align}
 This gives:
\begin{align}
P\left(\max_{k = 1,\ldots, \mathcal{N}} \delta_m^2 - ||\Delta_m^k||^2_T > (1 - \frac{\psi}{2} \omega) \delta_m^2 \right) \leq \exp \left(\frac{2048 U^2 \rho_m}{\gamma^2} k^2 \log(2 M k^2) - c \frac{\omega^2}{\rho_m^2 k^4} T \right).
\end{align}
By letting $\gamma = \frac{\xi \omega}{8}$ gives:
\begin{align}
P\left(\mathcal{Z}_T(\mathcal{B}_m) > ( 1- \frac{\xi}{4} \omega ) \delta^2_m \right) \leq \exp \left( \left( \frac{2^17 U^2 \rho_m}{\xi^2 \omega^2} \right) k^2 \log(2 M k^2) - \frac{ c \omega^2 T}{\rho_m^2 k^4} \right) \\
 &= \exp\left(\frac{c' \rho_m}{\omega^2} k^2 \log(2Mk^2) - \frac{c \omega^2 T}{\rho_m^2 k^4} \right).
\end{align}
Which implies that on $B'_{m}(\delta_m)$ we have that $||\Delta_m||_{T}^2 \geq \frac{ \xi \omega}{4} ||\Delta_m||_2^2 $ with high probability. Thus combining all three cases and the definition of $\rho_m = \frac{3}{\sigma} \lambda \sqrt{\rho_m}$
\begin{align}
\max (||\Delta_m||_F^2,||\Delta_m||_T^2) \leq \frac{144}{\sigma^2 \omega^2 \xi^2} \rho \lambda^2
\end{align}
with probability at least $1 -  \exp\left(\frac{c' \rho_m}{\omega^2} k^2 \log(2Mk^2) - \frac{c \omega^2 T}{\rho_m^2 k^4}\right)$.
\subsection{Lemmas}
\begin{lemma} \label{lemma_martingale}(Lemma 3.3 in \cite{}). Let $(Y_n, n \in \mathbb{N})$ be a martingale. For all $k \geq 2$, let 
\begin{align}
M_n^k = \sum_{i = 1}^{n}E[(Y_i - Y_{i-1})^k|\mathcal{F}_{i-1}].
\end{align}
Then for all integers $n \geq 1$ and for all $\eta$ such that for all $i \leq n$, $E[\exp(|\eta(Y_i - Y_{i-1})|)] \leq \infty$,
\begin{align}
\epsilon_n = \exp \left(\eta Y_n - \sum_{k \geq 2} \frac{\eta^k}{k!} M_n^k \right)
\end{align}
is a super-martingale. Additionally, if $Y_0 = 0$, then $E[\epsilon_n] \leq 1$.
\end{lemma}

\begin{lemma}
Let $\Delta_m$ be any element of $\mathcal{B}_{m}^{'}(\delta_m)$ defined in Eq. \refeq{}, and let the sequence $X_1, X_2, \ldots, X_T$ be randomly drawn according to the multivariate GLM autoregressive model in Eq. \refeq{}, and follow Assumption \ref{}. Then we have
\begin{align}
\mathbb{P}(\delta_m^2 - ||\delta_m^k||_T^2 > (1 - \frac{|\mathcal{T}}{2 T} \omega) \delta_m^2 ) \leq \exp \left(-c \frac{\omega^2}{\rho_m^2} \right)
\end{align}
for some $c \geq 0$ which is independent of $M, T, s$ and $\rho_m$.
\end{lemma} 
\emph{proof}
Define the sequence $(Y_n,n \in \mathbb{N})$ as
\begin{align}
Y_n = \frac{1}{T} \sum_{t = 1}^{n} E[||\Delta_m \Xt||_2^2|\Xto] - \frac{1}{T} \sum_{t = 1}^{n} ||\Delta_m \Xt||_2^2
\end{align}
Define
\begin{align}
Y_n - Y_{n-1} &= \frac{1}{T} E[||\Delta_m \Xt||_2^2||\Xno] - \frac{1}{T} ||\Delta_m \Xn||_2^2 \\
M_n^q &= \sum_{i=1}^n E \left[ \left( \frac{1}{T} E[||\Delta_m \Xt||_2^2|\Xto] - \frac{1}{T} ||\Delta_m \Xt||_2^2 \right)^q|X_{\mathcal{T}_1}, \ldots, \Xto \right].
\end{align}
The first value shows that $E\left[Y_n - Y_{n-1}|X_{\mathcal{T}_1}, \ldots, \Xto \right] = 0$ so that $Y_n$ is a martingale. \textcolor{red}{Additionally, on $\mathcal{T}$, we have that $0 \leq ||\Delta_m X_t||_2^2 \leq ||\Delta_m||_{1}^{2} ||X_t||_{\infty}^{2} \leq k^2 ||\Delta_m||_{\mathcal{\G}}^2 U^2$. Because $\Delta_m \in \mathcal{B}_m^{'}(\delta_m)$, it is true that $||\Delta_m||_{\G} \leq 4 || \Delta_{m,\mathcal{S}}||_{\G}$. By Cauchy Shwartz we have that $||\Delta_{m,\mathcal{S}}||_{\G} \leq \sqrt{\rho_m} ||\Delta_{m,\mathcal{S}}||_{F} \leq \sqrt{\rho_m} ||\Delta_{m}||_{F}$. This implies that $||\Delta_m X_t||_2^2 \leq 16 \rho_m k^2 \delta_m^2 U^2 = B$}. Therefore $|Y_n - Y_{n-1}| \leq \frac{B}{T}$ and
\begin{align}
M_n^q \leq n \left( \frac{B}{T} \right)^q
\end{align}
Using the summation term in Lemma \ref{lemma_martingale} gives the bound,
\begin{align}
D_n = \sum_{q \geq 2} \frac{\eta^{q}}{q!}M_n^q \leq n \sum_{q \geq 2} \frac{\eta^q B^q}{T^q q!} = n (e^{\eta B/T} - 1 - \frac{\eta B}{T}) = \hat{D}_n.
\end{align}
Markov's inequality gives the bound:
\begin{align}
P(Y_n \geq y) \leq E[e^{\eta Y_n}] e^{\eta y} = E[e^{\eta Y_n - D_n + D_n}] e^{-\eta y} \leq E[e^{\eta Y_n - D_n}] e^{\hat{D_n} - \eta y} \leq e^{\hat{D}_n - \eta y}
\end{align}
The final inequality comes from Lemma \ref{lemma_martingale}, which states that the terms are supermartingales with initial term equal to 1, so the entire expectation is less than or equal to one. Optimizine the bound for $\eta$ gives $\eta = \frac{T}{B} \log(\frac{T y}{n B} + 1)$, giving:
\begin{align}
P(Y_n \geq y) &\leq \exp{\left(n \left(\frac{T y}{n B} - \log\left(\frac{T y}{n B} + 1\right)\right) - \frac{T y}{B} \log \left(\frac{T y}{n B} + 1 \right) \right)} \\
&= \exp\left(- n H\left(\frac{T y}{n B} \right) \right)
\end{align}
whre $H(x) = (1 + x) \log(1 + x) - x$. We can use the fact that $H(x) \geq \frac{3 x^2}{2 (x + 3)}$ for $x \geq 0$ to get
\begin{align}
P(Y_n \geq y) \leq \exp \left(\frac{- 3 T^2 y^2}{2 B T y + 6 n B^2} \right)
\end{align}
Plugging in out value of $B$ and letting $n = |\mathcal{T}|$ gives 
\begin{align}
P\left(\frac{1}{T} \sum_{i = 1}^{|\mathcal{T}|} E [ ||\Delta_m \Xt||_2^2 | \Xto] - \frac{1}{T} \sum_{i = 1}^{\mathcal{T}} ||\Delta_m \Xt||_2^2 \geq y \right) \leq \left( - \frac{3 T y^2}{2^5 U^2 k^2 \rho_m \delta_m^2 y + 3*2^9 U^4 \rho_m^2 \delta_m^4 k^4} \right)
\end{align}
To get the final form of the Lemma, we lower bound the smallest eigenvalue of $E[\Xt \Xt^T|\Xt]$:
\textcolor{red}{
\begin{align}
\frac{1}{T} \sum_{i = 1}^{|\mathcal{T}|} E[||\Delta_m \Xt||_2^2 | \Xto] &= \sum_{t = 1}^{|\mathcal{T}|}  E[\Xt^T \Delta_m^T \Delta_m \Xt | \Xto] \\
&= \sum_{t = 1}^{|\mathcal{T}|} E [\text{trace} \left(\Xt^T \Delta_m^T \Delta_m \Xt | \Xto] \right)\\
&= \sum_{t = 1}^{|\mathcal{T}|}\text{trace} \left( \Delta_m E [\Xt \Xt^T | \Xto ]
\Delta_m^T \right) \\
&= \sum_{i = 1}^{|\mathcal{T}|} \sum_{j = 1}^{k} \Delta_{mj} E [\Xt \Xt^T | \Xto ] \Delta_{mj}^T \\
&\geq \sum_{i = 1}^{T} \sum_{j = 1}^{k} \omega ||\Delta_{mj}||_2^2 \\
&= \frac{|\mathcal{T}|}{T} \omega ||\Delta_{m}||_F^2 
\end{align}
where $\Delta_{mj}$ is the $j$th row of $\Delta_m$.}
Combining results gives:
\begin{align}
||\Delta_m||_T^2 \geq \frac{|\mathcal{T}|}{2T} \omega ||\Delta_m||_2^2 = \frac{|\mathcal{T}|}{2T} \omega \delta_m
\end{align}
with probability at least $1 - \exp\left(- \left(\frac{3 \psi^2}{2^6 U^2 + 3*2^{11} U^4 } \right) \frac{\omega^2 T}{\rho_m^2 k^4} \right)$.

\begin{lemma} \label{gauss_comp}
Let $(w_t)_{t = 0}^{T}$ be i.i.d k dimensional $\mathcal{N}(0,I)$ random variables which are also independent of $\{X_t\}_{t = 0}^T$, where $X_t \in [-U,U]^{Mk}$. Then
 \begin{align}
 E_w \left[\left|\left|\frac{1}{\sqrt{T}} \sum_{t \in \mathcal{T}} w_t X_t^T\right|\right|_{\G, \infty}\right] \leq U k \sqrt{2 \log (2 M k^2)}
 \end{align}
\end{lemma}
(\emph{Proof}) First we have that
\begin{align}
\left|\left|\frac{1}{\sqrt{T}} \sum_{t \in \mathcal{T}} w_t X_t^T\right|\right|_{\G, \infty} \leq k \left|\left|\frac{1}{\sqrt{T}} \sum_{t \in \mathcal{T}} w_t X_t^T\right|\right|_{\infty}.
\end{align}
Now $\sum_{t\in \mathcal{T}} X_{t,l} w_{t,j}$ is a normal random variable with mean zero and variance $\sum_{t \in \mathcal{T}} X_{t,l}^2$. We may use the following to bound the expected value of the maximum of a set of random variables:
\begin{align}
\exp \left(\beta E_w \left[\max_{1 \leq l \leq Mk, 1 \leq j \leq k} |\sum_{t\in \mathcal{T}} X_{t,l} w_{t,j}| \right] \right)
 &\leq E_w \left[ \max_{1\leq l \leq Mk, 1 \leq j \leq k} \exp \left( \beta |\max_{1\leq l \leq Mk, 1 \leq j \leq k}| \right) \right] \\
& \leq \sum_{l = 1}^{Mk} \sum_{j = 1}^k E_w \left[ \exp \left(\beta  \sum_{t\in \mathcal{T}} X_{t,l} w_{t,j} \right) + \exp \left( - \beta  \sum_{t\in \mathcal{T}} X_{t,l} w_{t,j} \right)\right] \\
&= 2 Mk^2 \exp \left(\beta^2 \sum_{t \in \mathcal{T}} X^2_{t,l}/2 \right)
\end{align}
Which follows by Jensen's inequality, monotonicity of exponential function, the sum of positive numbers being larger than the maximum, and the fact that $e^{|x|} \leq e^{-x} + e^{x}$, and the moment generating function for a normal random variable. Taking logs and setting $\beta = \sqrt{2 \log(2Mk^2)/\sum_{t \in \mathcal{T}} X_{t,l}^2}$ gives
\begin{align}
E_w \left[\max_{1\leq l \leq Mk} \max_{1\leq j \leq k} \left|\sum_{t \in \mathcal{T} }X_{l,t} w_{t,j}\right| \right] \leq  \sqrt{2 \log(2Mk^2) \sum_{t \in \mathcal{T}} X_{l,t}^2} \leq U \sqrt{2 T \log(2Mk^2)}
\end{align}
and dividing both sides by $\sqrt{T}$ proves the result.
\subsection{Categorical Distribution}
For the Categorical distribution with $k + 1$ categories we have the following autoregressive model:
\begin{align}
X_{t+1,m}|X_t \sim \text{Categorical}\left(\frac{1}{\text{exp}Z}\left(\text{exp}(\nu_{m,1} + \sum (A^*_{l,m})_1 X_{t,l}), \ldots, \text{exp}(\nu_{m,k} + \sum (A^*_{l,m})_k X_{t,l})\right)\right)  
\end{align}
where $Z = \log\left(1 + \sum_{i = 1}^{k} \text{exp}(\nu_{m,i} + \sum (A^*_{l,m})_i X_{t,l}\right)$. Note we let $X_{t+1,m}$ be a $k$ dimensional vector, where the all zero vector implies that category $k + 1$ was selected. Due to the Categorical distribution we have $\beta = 1$ and strong convexity parameter of $Z$ on the bounded range given by $ $.

\begin{ntheorem} \label{cat_th}
For a sequence generated from the Categorical autoregressive process with the matrix $A^*$ and $\nu$, we have the following properties:
\begin{enumerate}
\item \textcolor{red}{The smallest eigenvalue of the matrix $\Gamma_t = E[X_t X_t^T|X_{t-1}]$ is lower bounded by \begin{align}
\min \left(\frac{\exp\left(\tilde{\nu} + s k \tilde{a} \right)}{(1 + \exp(\tilde{\nu} + s k \tilde{a}))^{k+1} }, \frac{\exp\left(-\tilde{\nu} - s \tilde{a} \right)}{(1 + \exp(-\tilde{\nu} - s \tilde{a}))^{k+1} }\right)
\end{align}}
\item \textcolor{red}{The strong convexity parameter of $Z$ on the bounded range is lower bounded by
\begin{align}
 \min \left(\frac{\exp\left(\tilde{\nu} + s k \tilde{a} \right)}{(1 + \exp(\tilde{\nu} + s k \tilde{a}))^{k+1} }, \frac{\exp\left(-\tilde{\nu} - s \tilde{a} \right)}{(1 + \exp(-\tilde{\nu} - s \tilde{a}))^{k+1} }\right)
\end{align}
}
\item \textcolor{red}{Assuming $T \geq 2$ and $\log(Mk) \geq 1$ \begin{align}
\max_{1 \leq i,j \leq M} \frac{1}{T} \left|\left| \sum_{t = 0}^{T-1} \left(X_{t,i} - E(X_{t,i}|X_{t-1} \right) X^T_{t-1,j}\right|\right|_{F} \leq k \frac{3 \log(M k T)}{\sqrt{T}}
\end{align}
with probability at least $1 - \frac{1}{M k T}$.}
\end{enumerate}
\end{ntheorem}

\textcolor{red}{\subsection{Proof of Theorem \ref{cat_th}}
$\Gamma_t$ can be written as
\begin{align}
\Gamma_t = E[X_t|X_{t-1}] E[X_t|X_{t-1}]^T + \left( \begin{array}{c c c}
\text{Cov}(X_{t,1}|X_{t-1}) & \ldots & 0 \\
\vdots & \ddots & \vdots \\
0 & \ldots & \text{Cov}(X_{t,M}|X_{t-1})
\end{array} \right).
\end{align}
Where $Cov(X_{t,1} | X_{t-1})$ is the covariance matrix of a categorical distribution. We may lower bound $\Gamma_t$ by lower bounding $\text{Cov}(X_{t,1} | X_{t-1})$ since the first term is positive semidefinite. First note that we may derive the following bound for the smallest eigenvalue of a positive definite matrix $\Sigma$:
\begin{align}
|\Sigma| = \prod_{i = 1}^{k} \lambda_i
\leq (\lambda_{max})^{k-1} \lambda_{min}
\end{align}
so that 
\begin{align}
\lambda_{min} \geq \frac{|\Sigma|}{(\lambda_{max})^{k-1}}
\end{align}
Note that for a $k + 1$ categorical distribution with parameter $p$ where  $0 \leq p \leq 1$, $0 \leq  1 - 1^T p \leq 1$, the covariance matrix $\Sigma$ of the $k$ dimensional vector X is given by:
\begin{align}
\Sigma = \text{diag}(p) - p p^t
\end{align}
Note that the determinant is given by:
\begin{align}
|\Sigma| &= \prod_{i = 1}^k p_i  - \sum_{i = 1}^{n} p_i \prod_{i=1}^{k} p_i \\
&= \left(\prod_{i = 1}^k p_i \right) (1 - 1^T p) \\
\end{align} 
 Furthermore, $\lambda_{max} \leq 1$ so that 
\begin{align}
\lambda_{min} \geq \left(\prod_{i = 1}^k p_i \right) (1 - 1^T p)
\end{align}
For the autoregressive GLM the term on the right hand side is lower bounded, due to the bounded range of $A^*$ and of $X_t$, as
\begin{align}
\lambda_{min} &\geq \sigma \\
&= \min \left(\frac{\exp\left(\tilde{\nu} + s k \tilde{a} \right)}{(1 + \exp(\tilde{\nu} + s \tilde{a}))^{k+1} }, \frac{\exp\left(-\tilde{\nu} - s \tilde{a} \right)}{(1 + \exp(-\tilde{\nu} - s \tilde{a}))^{k+1} }\right)
\end{align}
for all $t$.}

\subsubsection{Part 2}
The strong convexity parameter $\kappa$ is also given by a lower bound on the eigenvalues of the Hessian of $Z(.)$ on the bounded range.
\textcolor{red}{The Hessian of $Z({\bf x}) = \log \left(1 + \sum_{i = 1}^{k} \exp(x_i)\right) := \log(L)$ may be written as:
\begin{align}
H = \frac{1}{\exp \left(2 Z({\bf x}) \right)} \left(\text{diag}\left(\exp({\bf x}) \exp(Z)\right) - \exp({\bf x}) \exp({\bf x})^T \right)\end{align}
The determinant is equal to:
\begin{align}
|H| &= \frac{1}{L^{2k}} \left(L^k\exp(\sum_{i = 1}^{k} x_i) - L^{k-1}\sum_{i = 1}^{k} \exp(x_i) \exp\left(\sum_{i = 1}^k x_i\right) \right) \\
&= \frac{L^{k-1} \exp\left(\sum_{i=1}^k x_i\right)}{L^{2k}} \left(L - \exp \left(\sum_{i = 1}^{k} x_i\right) \right) \\
&= \frac{\exp\left(\sum_{i=1}^k x_i\right)}{(1 + \exp(\sum_{i = 1}^{k} x_i))^{k+1} }
\end{align}
which on the bounded range implies that:
\begin{align}
\lambda_{min} &\geq \kappa \\
&= \min \left(\frac{\exp\left(\tilde{\nu} + s k \tilde{a} \right)}{(1 + \exp(\tilde{\nu} + s k \tilde{a}))^{k+1} }, \frac{\exp\left(-\tilde{\nu} - s \tilde{a} \right)}{(1 + \exp(-\tilde{\nu} - s \tilde{a}))^{k+1} }\right)
\end{align}
}

\subsubsection{Part 3}
\textcolor{red}{First we note that 
\begin{align}
\left|\left|\frac{1}{T}\sum_{t=0}^{T-1} \left(X_{t}^i - E[X_{t}^i|X_{t-1}]\right) (X_{t-1}^{j})^T\right|\right|_F \leq k\left|\left|\frac{1}{T}\sum_{t=0}^{T-1} \left(X_{t}^{i} - E[X_{t}^{i}|X_{t-1}]\right) (X_{t-1}^{j})^T\right|\right|_{\infty}
\end{align}
implying that 
\begin{align}
\max_{1 \leq i,j \leq M}  \left|\left| \frac{1}{T}\sum_{t = 0}^{T-1} \left(X_{t}^{i} - E[X_{t}^i|X_{t-1}] \right) (X_{t-1}^{j})^T\right|\right|_{F} \leq  k \max_{1 \leq m,l \leq Mk} \frac{1}{T}\left|\sum_{t = 0}^{T-1} (X_{t,m} - E(X_{t,m}|X_{t-1}) X_{t-1,l})\right|
\end{align}}
We now present the same argument as in Theorem 2 in \cite{Hall:2016} to the categorical case and we give the proof below for completeness.

Define the sequence $(Y_n, n \in \mathbb{N})$ as:
\begin{align}
Y_n = \frac{1}{T} \sum_{t=0}^{n-1} X_{t,m} (X_{t+1,l} - E[X_{t+1,l}|X_t]).
\end{align} 
and we have that
\begin{align}
Y_n - Y_{n-1} &= \frac{X_{n-1,m}}{T}(X_{i,l} - E[X_{i,l}|X_{i-1}]) \\
M_n^q &= \sum_{i=1}^n E\left[ \left( \frac{X_{i-1},m}{T} (X_{i,l} - E[X_{i,l}|X_{i-1}]) \right)^q | X_q, \ldots, X_{i-1} \right]
\end{align}
showing that $E[Y_n - Y_{n-1}|X_1, \ldots, X_{n-1}] = 0$ showing that $Y_n$ is a martingale. Additionally, we have that $|Y_n - Y_{n - 1}| \leq \frac{1}{T} = B$ and
\begin{align}
M^2_n &= \sum_{i = 1}^{n} E\left[\left(\frac{X_{t-1,m}}{T} (X_{i,l} - E[X_{i,l}|X_{i-1}])\right)^2 |X_1, \ldots, X_{i-1} \right] \\
&= \frac{1}{T^2} \sum_{i = 1}^n X^2_{i-1,m} E[(X_{i,l} - E[X_{i,l}|X_{i-1}])^2|X_{i-1}] \leq \frac{n}{4 T^2} :=  \hat{M}_n^2
\end{align}
which follows since each entry in the  Categorical random variable vector is bounded by one and has variance bounded by $\frac{1}{4}$. We can also bound $M_n^q$ as:
\begin{align}
M_n^q = \sum_{i = 1}^n E \left[ \left( \frac{X_{i-1,m}}{T} (X_{i,l} - E[X_{i,l}|X_{i-1}]) \right)^2 \left( \frac{X_{i-1,m}}{T} (X_{i,l} - E[X_{i,l}|X_{i-1}]) \right)^{q - 2} | X_{i-1} \right]
\leq B^{q - 2} M_n^2
\end{align}
We use this last result to get a bound on the $D_n$ terms used in the martingale results in Lemma \ref{lemma_martingale}. 
\begin{align}
D_n &:= \sum_{q \geq 2} \frac{\eta^q}{q!} M_n^q \leq \sum_{q \geq 2} \frac{\eta^q B^{q - 2} M^2_n}{q!} \leq \frac{\hat{M}^2_n}{B^2} \sum_{q \geq 2} \frac{(\eta B)^q}{q!} := \hat{D}_n \\
\tilde{D}_n &:= \sum_{q \geq 2} \frac{\eta^q}{q!} (-1)^q M_n^q \leq \hat{D}_n.
\end{align}
We use Markov's inequality to bound:
\begin{align}
P(|Y_n| \geq y) = P(Y_n \geq y) + P(-Y_n \geq y) \leq E[e^{\eta Y_n}] e^{- \eta y} + E[e^{\eta (-Y_n)} ] e^{-\eta y} \\
= E[e^{\eta Y_n - D_n + D_n}] e^{-\eta y} + E[e^{\eta (-Y_n) - \tilde{D}_n + \tilde{D}_n}] e^{- \eta y} \\
\leq E[e^{\eta Y_n - D_n}]e^{\hat{D}_n - \eta y} + E[e^{\eta (-Y_n) - \tilde{T}_n}]e^{\hat{D}_n - \eta y} \leq 2 e^{\hat{D}_n - \eta y}.
\end{align}
Where the final inequality comes from Lemma \ref{lemma_martingale} since the terms are super martinagales with first term being 1, so the expectation is less than or equal to one. Setting $\eta = \frac{1}{B} \log(\frac{y B}{\hat{M}_n^2})$ yields the lowest bound, giving:
\begin{align}
P(|Y_n| \geq y) \leq 2 \exp \left(- \frac{\hat{M}_n^2}{B^2} H \left(\frac{y B}{\hat{M}_n^2} \right) \right) 
\end{align}
where $H(x) = (1 + x) \log(1 + x) - x$. We use the fact that $H(x) \geq \frac{3 x^2}{2 (x + 3)}$ for $x \geq 0$ to simplify the bound:
\begin{align}
P(|Y_n| \geq y) \leq 2 \exp \left( \frac{-3 y^2}{2 y B + 6 \hat{M}^2_n} \right) = 2 \exp \left( - \frac{6 y^2 T^2}{4 y T + 3n} \right)
\end{align}
\textcolor{red}{Setting $n = T$ and taking a union bound over all indices gives:
\begin{align}
& P \left(  \max_{1 \leq l, m \leq Mk} \frac{1}{T} \left|\sum_{t = 0}^{T-1} X_{t-1,l} (X_{t,m} - E[X_{t,m}|X_{t-1}]) \right| \geq 3 \frac{\log M k T}{\sqrt{T}} \right) \\
&\leq \exp \left(\log (2 M^2 k^2) - \frac{ 54 \log (M k T)}{\frac{12}{\sqrt{T}} + 3} \right) \\
&\leq \frac{1}{M k T}
\end{align}
Where we assumed $T \geq 2$ and $\log(MkT) \geq 1$. Together this implies that
\begin{align}
&P \left(\max_{1 \leq i,j \leq M}  \left|\left| \frac{1}{T}\sum_{t = 0}^{T-1} \left(X_{t}^{i} - E[X_{t}^i|X_{t-1}] \right) (X_{t-1}^{j})^T\right|\right|_{F} \geq 3 k \frac{\log M k T}{\sqrt{T}} \right)\\
&\leq \frac{1}{M k T}
\end{align}}
